# Supplementary material for: Variance Penalized On-Policy and Off-Policy Actor-Critic
Source: arXiv:2102.01985 source file (2021-02-03)
Supplement: Supplementary file 1 [file estimationerrorvariance.tex]

\section{Estimation error in the variance}
In this section, we show that when the approximate state-action value function $\hat Q(s,a)$ is used in the variance function recursion \eqref{sigma_org_onpac}, instead of the true state-action value function $Q_\pi(s,a)$, then the estimation error in the variance is bounded under certain conditions. In this section, we do not claim any novelty for the on-policy estimation error bound on the variance . The proof for Theorem \ref{thm:err_var_onp} is taken from \cite{sherstan2018directly} (Theorem 2, proved with value function $V(s)$ instead of state-action value function $Q(s,a)$) and expanded here for the sake of completeness and consistency of the notations. On the similar lines, we show the estimation error bound for the off-policy variance in Theorem \ref{thm:err_var_offp}.

\begin{theorem}\label{thm:err_var_onp}(\textbf{Error bound for on-policy variance}):
The estimate of the variance is represented by $\hat \sigma(s,a) =  \E_\pi[\delta_t^2 + \gamma_{t+1}^2 \hat \sigma(S_{t+1},A_{t+1})| S_t = s, A_t =a]$. If the squared estimation error of state-action value function is bounded by $ (\hat Q(s,a) - Q_\pi(s,a))^2 \leq \epsilon(s,a)$ and accumulating error is  also bounded
\begin{equation*}
    \begin{split}
        \Big| \E_\pi\Big[\delta_{t}\gamma_{t+1}& (Q_\pi(S_{t+1},A_{t+1}) - \hat Q(S_{t+1},A_{t+1}))|S_t =s, A_t =a\Big] \\
        & + \E_\pi\Big[ \delta_{t+1}\gamma_{t+1}^2\gamma_{t+2}(Q_\pi(S_{t+2},A_{t+2}) - \hat Q(S_{t+2},A_{t+2}))|S_t =s, A_t =a\Big] + \dots \Big| \leq \epsilon(s,a),
    \end{split}
\end{equation*}
then the estimation error of the variance is also bounded.

\end{theorem}
\begin{proof}
The return in the discounted setting is denoted as \[G_{t} = R_{t+1} + \gamma_{t+1} G_{t+1}.\]
\begin{align*}
    \sigma_\pi(s,a) =& \E_\pi[(G_t - Q_\pi(s,a))^2 | S_t =s, A_t =a]\\
    =&\E_\pi[(G_t - Q_\pi(s,a) + \hat Q(s,a) - \hat Q(s,a) )^2 | S_t =s, A_t =a]\\
    =&\E_\pi[(G_t - \hat Q(s,a))^2| S_t =s, A_t =a] + (\hat Q(s,a) - Q_\pi(s,a) )^2\nonumber\\
    &+ 2\E_\pi[(G_t - \hat Q(s,a))| S_t =s, A_t =a](\hat Q(s,a) - Q_\pi(s,a) )
\end{align*}
The last term can be simplified to,
\begin{align*}
\E_\pi[(G_t - \hat Q(s,a))| S_t =s, A_t =a] =& \E_\pi[(G_t - Q_\pi(s,a))| S_t =s, A_t =a] + (Q_\pi(s,a) - \hat Q(s,a))\\
=&(Q_\pi(s,a) - \hat Q(s,a)).
\end{align*}
Therefore, the variance is simplified as,
\begin{align}\label{error_var}
    \sigma_\pi(s,a) =& \E_\pi[(G_t - \hat Q(s,a))^2| S_t =s, A_t =a]+ (\hat Q(s,a) - Q_\pi(s,a) )^2 - 2(\hat Q(s,a) - Q_\pi(s,a))^2\nonumber\\
    =& \E_\pi[(G_t - \hat Q(s,a))^2| S_t =s, A_t =a] -(\hat Q(s,a) - Q_\pi(s,a) )^2
\end{align}
Now we will simplify $\E_\pi[(G_t - \hat Q(s,a))^2| S_t =s, A_t =a]$ term. The TD error here is \[\delta_{t}(S_{t}, A_{t}, S_{t+1},A_{t+1}) = R_{t+1}} + \gamma_{t+1} \hat Q(S_{t+1},A_{t+1}) - \hat Q(S_{t}, A_{t}).\] We will from now on denote TD error as just $\delta_{t}$.
\begin{equation*}
\begin{split}
    \E_\pi[(G_t &- \hat Q(s,a))^2| S_t =s, A_t =a] \\
    =&\E_\pi\Big[\Big(\underline{R_{t+1}} + \gamma_{t+1} G_{t+1} \underline{- \hat Q(s,a) + \gamma_{t+1} \hat Q(S_{t+1},A_{t+1})} \\&\quad- \gamma_{t+1} \hat Q(S_{t+1},A_{t+1})\Big)^2| S_t =s, A_t =a\Big]\\
    =&\E_\pi[\big(\underline{\delta_{t}} + \gamma_{t+1}( G_{t+1} -\hat Q(S_{t+1},A_{t+1}))\big)^2| S_t =s, A_t =a]\\
    =&\E_\pi[\delta_{t}^2 | S_t =s, A_t =a]  + 2\E_\pi[\delta_{t}\gamma_{t+1} (G_{t+1} -\hat Q(S_{t+1},A_{t+1}))|S_t =s, A_t =a]\\
    &+ \E_\pi[\gamma_{t+1}^2\big( G_{t+1} -\hat Q(S_{t+1},A_{t+1})\big)^2| S_t =s, A_t =a]\\
    =&\E_\pi[\delta_{t}^2 | S_t =s, A_t =a] + 2\E_\pi[\delta_{t}\gamma_{t+1} (G_{t+1} -\hat Q(S_{t+1},A_{t+1}))|S_t =s, A_t =a]\\
    & +  \E_\pi\Big[\gamma_{t+1}^2\Big(R_{t+2} + \gamma_{t+2} G_{t+2}  - \hat Q(S_{t+1},A_{t+1}) \\&\quad + \gamma_{t+2} \hat Q(S_{t+2},A_{t+2}) - \gamma_{t+2} \hat Q(S_{t+2},A_{t+2})\Big)^2|  S_t =s, A_t =a\Big] \\
    =&\E_\pi[\delta_{t}^2 | S_t =s, A_t =a] + 2\E_\pi[\delta_{t}\gamma_{t+1} (G_{t+1} -\hat Q(S_{t+1},A_{t+1}))|S_t =s, A_t =a]\\
    & +  \E_\pi\Big[ {\gamma_{t+1}^2}\Big( {\delta_{t+1}} + \gamma_{t+2} (G_{t+2} - \hat Q(S_{t+2},A_{t+2}))\Big)^2|  S_t =s, A_t =a\Big]\\
    =&\E_\pi[\delta_{t}^2 +  {\gamma_{t+1}^2 \delta_{t+1}^2}| S_t =s, A_t =a] + 2\E_\pi[\delta_{t}\gamma_{t+1} (G_{t+1} -\hat Q(S_{t+1},A_{t+1}))|S_t =s, A_t =a]\\
    & +  2\E_\pi[ {\delta_{t+1}\gamma_{t+1}^2 }\gamma_{t+2}(G_{t+2} -\hat Q(S_{t+2},A_{t+2}))|S_t =s, A_t =a] \\
    & + \E_\pi[\gamma_{t+1}^2\gamma_{t+2}^2\big( G_{t+2} -\hat Q(S_{t+2},A_{t+2})\big)^2| S_t =s, A_t =a]\\
    =&\E_\pi[\delta_{t}^2 + \gamma_{t+1}^2  {\hat \sigma(S_{t+1}, A_{t+1})}| S_t =s, A_t =a] \\&\quad + 2\Big(\E_\pi[\delta_{t}\gamma_{t+1} (G_{t+1} -\hat Q(S_{t+1},A_{t+1}))|S_t =s, A_t =a]\\&\quad\quad +  \E_\pi[\delta_{t+1}\gamma_{t+1}^2\gamma_{t+2}(G_{t+2} -\hat Q(S_{t+2},A_{t+2}))|S_t =s, A_t =a] + \dots \Big)
\end{split}
\end{equation*}
On expanding one of the cross term above, 
\begin{align*}
    |\E_\pi[&\delta_{t}\gamma_{t+1} (G_{t+1} -\hat Q(S_{t+1},A_{t+1}))|S_t =s, A_t =a]| \nonumber\\
    = |&\underbrace{\E_\pi[\delta_{t}\gamma_{t+1} (G_{t+1} -Q_\pi(S_{t+1},A_{t+1}))|S_t =s, A_t =a]}_{=0} \\
    &+ \E_\pi[\delta_{t}\gamma_{t+1} (Q_\pi(S_{t+1},A_{t+1}) - \hat Q(S_{t+1},A_{t+1}))|S_t =s, A_t =a]|
\end{align*}
The first term in the above equation is zero using to Lemma \eqref{off_policy_cross_term}. The Equation \eqref{error_var} is now expressed as:
\begin{equation*}
\begin{split}
    \sigma_\pi(s,a) =\E_\pi[(G_t - \hat Q(s,a))^2| S_t =s, A_t =a] &-(\hat Q(s,a) - Q_\pi(s,a) )^2\\
    |\sigma_\pi(s,a) - \E_\pi[\delta_{t}^2 + \gamma_{t+1}^2 \hat \sigma(S_{t+1}, A_{t+1})| S_t =s, A_t =a]| &\leq |2 \times \text{Acc. error} + (\hat Q(s,a) - Q_\pi(s,a) )^2|\\
    |\sigma_\pi(s,a) - \hat \sigma(s,a)|& \leq |3\epsilon(s,a)|.
\end{split}
\end{equation*}
\end{proof}

\begin{theorem}\label{thm:err_var_offp} (\textbf{Error bound for off-policy variance}):
The estimate of the variance be represented by $\hat \sigma(s,a) =  \E_b[\delta_{t,\pi}^2 + \gamma_{t+1}^2 \rho_{t+1}^2\hat \sigma(S_{t+1},A_{t+1})| S_t = s, A_t =a]$. If the squared estimation error of value function is bounded by $ (\hat Q(s,a) - Q_\pi(s,a))^2 \leq \epsilon(s,a)$ and accumulating error is bounded
\begin{equation*}
    \begin{split}
        \Big| \E_\pi\Big[\delta_{t,\pi}&\gamma_{t+1}\rho_{t+1} (Q_\pi(S_{t+1},A_{t+1}) - \hat Q(S_{t+1},A_{t+1}))|S_t =s, A_t =a\Big] \\
        &\quad + \E_\pi\Big[ \delta_{t+1,\pi}\gamma_{t+1}^2\rho_{t+1}^2 \gamma_{t+2}\rho_{t+2}(Q_\pi(S_{t+2},A_{t+2}) - \hat Q(S_{t+2},A_{t+2}))|S_t =s, A_t =a\Big] \\
        &\quad\quad + \dots \Big| \leq \epsilon(s,a),
    \end{split}
\end{equation*}
then the estimation error of the variance is also bounded.
\end{theorem}

\begin{proof}
Similar to the Equation \eqref{error_var} in Theorem \ref{thm:err_var_onp}, the variance can be expressed as:
\begin{align}\label{error_var_offp}
    \sigma_\pi(s,a) = \E_b[(G_{t,\pi} - \hat Q(s,a))^2| S_t =s, A_t =a] -(\hat Q(s,a) - Q_\pi(s,a) )^2
\end{align}
The TD error here is \[\delta_{t,\pi} = R_{t+1} + \rho_{t+1} \gamma_{t+1} \hat Q(S_{t+1},A_{t+1}) -  \hat Q(S_{t}, A_{t}).\] On simplifying $\E_b[(G_{t,\pi} - \hat Q(s,a))^2| S_t =s, A_t =a]$ term,
\begin{equation*}
\begin{split}
    \E_b[&(G_{t,\pi} - \hat Q(s,a))^2| S_t =s, A_t =a] \\
    =&\E_b\Big[\Big(R_{t+1} + \gamma_{t+1}\rho_{t+1} G_{t+1,\pi} - \hat Q(s,a) \\&\quad+ \gamma_{t+1} \rho_{t+1} \hat Q(S_{t+1},A_{t+1}) - \gamma_{t+1}\rho_{t+1} \hat Q(S_{t+1},A_{t+1})\Big)^2| S_t =s, A_t =a\Big]\\
    =&\E_b[\big(\delta_{t,\pi} + \gamma_{t+1}\rho_{t+1}( G_{t+1,\pi} -\hat Q(S_{t+1},A_{t+1}))\big)^2| S_t =s, A_t =a]\\
    =&\E_b[\delta_{t,\pi}^2 | S_t =s, A_t =a]  + 2\E_b[\delta_{t,\pi}\gamma_{t+1}\rho_{t+1} (G_{t+1,\pi} -\hat Q(S_{t+1},A_{t+1}))|S_t =s, A_t =a]\\
    &+ \E_b[\gamma_{t+1}^2\rho_{t+1}^2\big( G_{t+1,\pi} -\hat Q(S_{t+1},A_{t+1})\big)^2| S_t =s, A_t =a]\\
    =&\E_b[\delta_{t,\pi}^2 | S_t =s, A_t =a] + 2\E_b[\delta_{t,\pi}\gamma_{t+1}\rho_{t+1} (G_{t+1,\pi} -\hat Q(S_{t+1},A_{t+1}))|S_t =s, A_t =a]\\
    & +  \E_b\Big[ {\gamma_{t+1}^2\rho_{t+1}^2}\Big( {\delta_{t+1,\pi}} + \gamma_{t+2} \rho_{t+2}(G_{t+2,\pi} - \hat Q(S_{t+2},A_{t+2}))\Big)^2|  S_t =s, A_t =a\Big]\\
    =&\E_b[\delta_{t,\pi}^2 +  {\gamma_{t+1}^2\rho_{t+1}^2 \delta_{t+1,\pi}^2}| S_t =s, A_t =a] \\&\quad + 2\E_b[\delta_{t,\pi}\gamma_{t+1}\rho_{t+1} (G_{t+1,\pi} -\hat Q(S_{t+1},A_{t+1}))|S_t =s, A_t =a]\\&\quad
     +  2\E_b[ {\delta_{t+1,\pi}\gamma_{t+1}^2\rho_{t+1}^2 }\gamma_{t+2}\rho_{t+2}(G_{t+2,\pi} -\hat Q(S_{t+2},A_{t+2}))|S_t =s, A_t =a] \\&\quad
     + \E_b[(\gamma_{t+1}\gamma_{t+2}\rho_{t+1}\rho_{t+2})^2\big( G_{t+2,\pi} -\hat Q(S_{t+2},A_{t+2})\big)^2| S_t =s, A_t =a]\\
    =&\E_b[\delta_{t,\pi}^2 + \gamma_{t+1}^2\rho_{t+1}^2  {\hat \sigma(S_{t+1}, A_{t+1})}| S_t =s, A_t =a] \\&\quad + 2\Big(\E_b[\delta_{t,\pi}\gamma_{t+1}\rho_{t+1} (G_{t+1,\pi} -\hat Q(S_{t+1},A_{t+1}))|S_t =s, A_t =a]
    \\&\quad\quad  +  \E_b[\delta_{t+1,\pi}\gamma_{t+1}^2\rho_{t+1}^2\gamma_{t+2}\rho_{t+2}(G_{t+2,\pi} -\hat Q(S_{t+2},A_{t+2}))|S_t =s, A_t =a] + \dots \Big)
\end{split}
\end{equation*}
On expanding one of the cross term above, 
\begin{align*}
    |\E_b[&\delta_{t,\pi}\gamma_{t+1}\rho_{t+1} (G_{t+1,\pi} -\hat Q(S_{t+1},A_{t+1}))|S_t =s, A_t =a]| \nonumber\\
    = |&\underbrace{\E_b[\delta_{t,\pi}\gamma_{t+1}\rho_{t+1} (G_{t+1,\pi} -Q_\pi(S_{t+1},A_{t+1}))|S_t =s, A_t =a]}_{=0} \\
    &+ \E_b[\delta_{t,\pi}\gamma_{t+1} \rho_{t+1}(Q_\pi(S_{t+1},A_{t+1}) - \hat Q(S_{t+1},A_{t+1}))|S_t =s, A_t =a]|
\end{align*}
The first term in the above equation is zero using to Lemma \eqref{off_policy_cross_term}. The \eqref{error_var_offp} can now be expressed as:
\begin{align*}
    \sigma_\pi(s,a) =\E_b[(G_{t,\pi} - \hat Q(s,a))^2| S_t =s, A_t =a] &-(\hat Q(s,a) - Q_\pi(s,a) )^2\\
    |\sigma_\pi(s,a) - \E_b[\delta_{t,\pi}^2 + \gamma_{t+1}^2\rho_{t+1}^2 \hat \sigma(S_{t+1}, A_{t+1})| S_t =s, A_t =a]| &\leq 2 \times \text{Acc. error} + (\hat Q(s,a) - Q_\pi(s,a) )^2\\
    |\sigma_\pi(s,a) - \hat \sigma(s,a)|& \leq |3\epsilon(s,a)|.
\end{align*}
\end{proof}
